# Supplementary material for: Elucidating the Origin of Heterogeneous Anomalous Diffusion in the Cytoplasm of Mammalian Cells
Source: arXiv:1910.00102 source file (2020-07-05)
Supplement: Supplementary file 1 [file adalPRL_suppl_final.pdf]

# Elucidating the origin of heterogeneous anomalous diffusion in the cytoplasm of mammalian cells
# – Supplementary Information –


Adal Sabri and Matthias Weiss
*Experimental Physics I, University of Bayreuth, Universitätsstr. 30, D-95447 Bayreuth, Germany*

Xinran Xu
*Department of Electrical and Computer Engineering,*
*Colorado State University, Fort Collins, CO 80523, USA*

Diego Krapf
*Department of Electrical and Computer Engineering,*
*Colorado State University, Fort Collins, CO 80523, USA and*
*School of Biomedical Engineering, Colorado State University, Fort Collins, CO 80523, USA*


**Contents**


**I. Materials and Methods** 1
A. Cell culture 1
B. Imaging 2
C. Single particle tracking and trajectory analysis 2
D. Resampling analysis of MSDs 3
E. Bootstrapping and averaging 3
F. Local convex hull analysis 4
G. Autocorrelation of squared increments 4
H. Simulations 5
I. Discussion of alternative model descriptions 5

**II. Supplementary figures** 7

**References** 12


## I. MATERIALS AND METHODS

### A. Cell culture

HeLa (human cervical cancer) cells were cultured in Dulbecco's Minimal Essential Medium (DMEM; Invitrogen, Carlsbad, CA) with phenol red, supplemented with 10% fetal calf serum (FCS; Biochrom, Holliston, MA) and 1% penicillin/streptavidin (ThermoFisher, Gibco, Waltham, MA) and incubated in Corning tissue-culture treated culture dishes at 37°C in a 5% $CO_2$ atmosphere. For imaging, cells were plated on 35 mm diameter ΔT dishes (Bioptech, Butler, PA) with ITO coating for temperature control. Prior to plating, dishes were coated with 0.5% matrigel matrix ($c_{\text{protein}} = 8 - 12$ mg/ml; Corning Life Sciences, NY) in Opti-MEM (ThermoFisher, Gibco, Waltham, MA). Experiments were performed 36-48 h after seeding.

Microtubule depolymerization was performed on the day of the experiment using nocodazole as described before [1–3]. Prior to microtubule breakdown, tracer particles (Qdot 655 ITK Carboxyl core (CdSe)-shell (ZnS), ThermoFisher, Waltham, MA) provided as 8 $\mu$M solution in 50 mM borate, pH 9.0 (working concentration 1:1000 in PBS with 1% BSA) were incorporated to the cytoplasm by the bead-loading technique [4] using 100 $\mu$m diameter glass beads (G4649-100G, Sigma Aldrich, St. Louis, MO). After bead loading, cells were incubated for another 45 min at 37°C. Glass beads were washed off gently with PBS and DMEM without phenol red, supplemented with 0.1% nocodazole ($c_{\text{stock}} = 10$ mM in DMSO). The dish was stored on ice for 10 min prior to 15 min recovery at 37°C in a 5% $CO_2$ atmosphere before performing the experiments.

Depolymerization of actin filaments was achieved using latrunculin A or cytocalasin D, respectively. On the day of the experiment, cells were loaded with quantum dots as described before and recovered for 45 min at 37°C. Glass

beads were washed gently with PBS and cells were incubated in DMEM without phenol red, supplemented with 200 nM latrunculin A or 2 $\mu$M cytocalasin D for another 30 min at 37°C prior to the experiments.

Treatment with filipin was performed with a protocol adapted from [5]: Filipin III (from *Streptomyces filipinensis* $\geq$ 85% HPLC; Sigma Aldrich), diluted to a working concentration of 15 $\mu$g/ml in imaging medium, was applied during bead loading and imaging. Hence, cells were exposed to filipin at least 30 min prior to and during particle-tracking experiments. The resulting breakdown of the ER network, in agreement with previous reports [5], was checked by fluorescence imaging with calreticulin-GFP (Addgene plasmid No. 80978) as described earlier [2]; see Fig. 4 (main text) for representative images.

Osmotic swelling was performed by applying diluted imaging medium (1:20 in pure water) as described in [6]. The resulting formation of polydisperse ER vesicles (imaged again with calreticulin-GFP, Fig. 4c) was comparable to previous observations in which cells had been shown to remain viable for many hours [6].

### B. Imaging

Images were acquired using Nikon NIS-Elements 4.51 software in a custom-built microscope equipped with an Olympus PlanApo 100× NA1.45 objective and a CRISP ASI autofocus system [7]. Optical aberrations of the imaging system were corrected using a MicAO 3DSR adaptive optics system (Imagine Optic, Orsay, France) inserted into the emission pathway between the microscope and the EMCCD camera [8]. The sample temperature was kept at 37°C using a Bioptechs stage heater. Quantum dots were excited with a 561-nm laser (OBIS 561nm LS 100mW, Coherent, Santa Clara, CA) under continuous illumination. For excitation, an optical density filter with ND=1 was used and an incident angle below the critical angle was chosen to provide a penetration depth of multiple micrometers. Emission was collected through the appropriate Semrock bandpass filters and images were acquired in a water-cooled, back-illuminated EMCCD camera (iXon DU-888, Andor, Belfast, UK) operated at −85°C at a rate of 10 frames/s over a total period of 2000 frames. Bright field images of the cells were also acquired prior to and after imaging.

Experiments on the effect of filipin were done together with controls on untreated cells on a laser scanning confocal microscope (Leica SP5, Leica Microsystems, Germany) using a 63x/1.4 oil immersion objective (HCX PL APO lambda blue 63x/1.4NA oil IMM) and an illumination at 476 nm. Fluorescence was detected in the range 630-680 nm and the bi-directional scan speed was adjusted to a frame time of 100 ms with an image size of $256 \times 256$ pixels ($41 \times 41$ $\mu$m$^2$).

### C. Single particle tracking and trajectory analysis

Trajectories were extracted from image stacks with FIJI/TrackMate [9]. As an input for TrackMate, the blob diameter of Qdots was estimated via the intensity profiles of 30 quantum dots immobilized on a coverslip, yielding an average FWHM of the point-spread function of $3.2 \pm 0.5$ pixels. Tracking was performed using the Laplacian-of-Gaussian algorithm (blob diameter set to 4 pixels, threshold set to 200, median filter and sub-pixel localization switched on). No additional filters were applied to the detected spots. Identified particle positions were linked using the *simple LAP (linear assignment problem)* tracker adopted from Ref. [10]. A maximum linking distance of 2 pixels, a gap-closing maximum distance of 2 pixels, and a gap closing maximum frame gap of 2 were used. Subsequently the minimum number of spots in a track was set to $N \geq 50$ and the number of gaps was set to $n_g \leq 5$. The spot statistics and the tracks were extracted and exported as CSV and XML files, respectively. Tracks were converted to ASCII files in Matlab for subsequent processing and handling. Statistical analyses of trajectories ($N$ positions with time lag $\Delta t$ between successive frames) were performed in Matlab with custom-written codes that have been checked for proper function via FBM simulation data. Trajectories whose TA-MSD grew less than $\sim \tau^{0.075}$ were rated as immobile and were hence discarded from subsequent analyses. In total, $n$ = 83, 57, 49, 75 cells (untreated or with nocodazole, cytochalasin D, latrunculin A, respectively) were used from which 4887, 9298, 2968, 3997 trajectories with $N = 100$ positions and 631, 841, 444, 517 trajectories with $N = 500$ positions were extracted. PDF bin sizes have been chosen according to Scott's rule throughout the manuscript.

As a control, we tracked quantum dots in cells treated with pure DMSO solvent without nocodazole, cytochalasin, or latrunculin. From five cells with 228 trajectories ($N = 100$) we obtained a mean anomaly $\langle\alpha\rangle = 0.65$ which is insignificantly higher than the value found for untreated cells. If DMSO has any effect, then it is rather a slight increase in $\langle\alpha\rangle$ whereas nocodazole led to a significantly smaller value. We therefore conclude that our results are not an artifact of DMSO.

As an additional control we also tracked quantum dots in purely viscous fluids, namely in (i) pure glycerol (viscosity $\eta \approx 1$ Pa s) and in (ii) aqueous sucrose solution (60% m/v, viscosity $\eta \approx 50$ mPa s). In both cases we observed a vanishing anomaly, i.e. we obtained $\langle\alpha\rangle = 1 \pm 0.05$ by the bootstrapping approach for both, geometric and arithmetic averaging. Data for glycerol are shown in Fig. S2f,g). Due to the different viscosities, the average diffusion coefficients

were $D = 0.015\mu\mathrm{m}^2/\mathrm{s}$ in glycerol and $D = 0.25\ \mu\mathrm{m}^2/\mathrm{s}$ for 60%-sucrose solution. Moreover, the anti-persistence-related minimum of the rescaled VACF at $\tau/\delta t = 1$ was negligible ($|C_v(\tau/\delta t \geq 1)| < 0.05$), as expected for normal diffusion. These data confirm that the emergence of a diffusion anomaly in cells is not an evaluation or measurement artifact due to a particularly slow normal diffusion.

Additional confocal image series for quantum dots in untreated, filipin-treated, and osmotically shocked cells were recorded and tracked as described above, yielding 366, 295, and 81 trajectories of length $N = 100$, respectively. Due to cellular background fluorescence and the lower pixel integration time (as compared to camera-based tracking) we observed a significant positive offset in the resulting TA-MSDs at small times. Therefore, the simple fitting and bootstrapping approach was not appropriate to evaluate these data. Instead, we utilized a recently introduced and validated resampling approach [11] (described in the next subsection) that eliminates all localization offsets.

### D. Resampling analysis of MSDs

In order to extract a meaningful average scaling exponent $\langle\alpha\rangle$ from TA-MSDs with static localization errors, we exploited a recently introduced and validated resampling approach (see [11] for details). In particular, we first calculated for each trajectory $\mathbf{r}(i\Delta t)$ $(i = 1, \ldots, N)$ the usual TA-MSD, $\langle r^2(\tau)\rangle_t$ with $\tau/\Delta t = 1, 2, \ldots$ which yielded the quantity $v(\tau, \Delta t) = \langle r^2(\tau)\rangle_t - \langle r^2(\Delta t)\rangle_t$ upon subtracting the first value. Then, we considered only the even or the odd positions of the very same trajectory and calculated from these $N/2$ positions the two TA-MSDs with lag times $\tau/\Delta t = 2, 4, \ldots$. Averaging these two TA-MSDs and subtracting the first value yielded $v(\tau, 2\Delta t)$. Since $v(\tau, k\Delta t) = k^\alpha v(\tau, \Delta t)$, the ratio of these functions can be used to extract $\langle\alpha\rangle$ without fitting [11]:

$$\langle\alpha\rangle = \frac{1}{\log(2)}\left\langle \log\left(\frac{\langle v(\tau, 2\Delta t)\rangle_g}{\langle v(\tau, \Delta t)\rangle_g}\right)\right\rangle_\tau \quad (1)$$

where $\langle . \rangle_g$ denotes a geometric averaging over trajectories and $\langle . \rangle_\tau$ indicates an averaging over lag times $\tau \leq 10\Delta t$.

Applying this evaluation approach to our camera-based tracking data ($N = 100$) confirmed the results given in Table 1 of the main text, e.g. $\langle\alpha\rangle = 0.59$ and $\langle\alpha\rangle = 0.39$ for untreated and nocodazole-treated cells.

Evaluating tracking data from confocal image series yielded a slightly higher value for untreated cells ($\langle\alpha\rangle = 0.68$), likely due to the measurement process with a moving focus in the confocal imaging. Filipin-treated and osmotically-shocked cells showed mean anomalies that were consistent with untreated cells, with a tendency for lower and elevated values, $\langle\alpha\rangle = 0.59$ and $\langle\alpha\rangle = 0.72$, respectively. Given that both treatments lead to a fragmented ER, we cannot conclude a significant change of $\langle\alpha\rangle$ when the ER network structure is lost.

### E. Bootstrapping and averaging

For the bootstrapping approach, we used the following scheme: Based on a total set of several hundred TA-MSDs, from individual trajectories for a given condition, we randomly selected $n = 100$ trajectories and averaged these to a single, sub-ensemble averaged TA-MSD from which we determined the scaling exponent $\alpha$. This random drawing from the total set of TA-MSDs and the subsequent averaging was repeated 200 times to obtain a PDF for the values of $\alpha$ (displayed in Fig. 1a of the main text and in Fig. S1).

For creating each sub-ensemble-averaged MSD, we used either a simple arithmetic averaging of individual TA-MSDs $\langle r^2(\tau)\rangle_t^{(i)}$ $(i = 1, \ldots, n)$ or a geometric averaging, i.e.

$$\langle r^2(\tau)\rangle_{t,g} = \left(\prod_{i=1}^{n} \langle r^2(\tau)\rangle_t^{(i)}\right)^{1/n} . \quad (2)$$

We would like to note here that the logarithmic of Eq. (2) is similar to the mean-log-square displacement proposed by Kepten et al. [12] to reduce systematic errors in the estimation of $\langle\alpha\rangle$,

$$\log\left[\left(\prod_{i=1}^{n} \langle r^2(\tau)\rangle_t^{(i)}\right)^{1/n}\right] = \frac{1}{n}\sum_{i=1}^{n} \log\langle r^2(\tau)\rangle_t^{(i)}. \quad (3)$$

Using MSDs obtained from the bootstrapping approach with geometric averaging we also explored the magnitude of potential TA-MSD offsets induced by localization errors. To this end, we calculated the difference between the experimental MSD and its simple, offset-free fit $K_\alpha\tau^\alpha$ at $\tau = \Delta t$ (where the influence of localization errors should be strongest). As a result, we observed in all cases only a very small positive difference $c$, indicating a positive offset in the experimental MSD, that was significantly lower than the diffusional contribution, i.e. $c/(K_\alpha \Delta t^\alpha) < 5\%$.

## F. Local convex hull analysis

In order to directly visualize changes in the mobility within single trajectories, we employed the local convex hull (LCH) [13]. The integral-like character of this approach requires less statistics within the trajectories as compared to a local TA-MSD analysis that has proven useful for dissecting diffusive and ballistic motion [14]. For consistency with the PDF of normalized increments, $p(\chi)$, we rescaled all trajectories with $N = 100$ by their respective average displacement at the minimal length scale, $\Delta r = \sqrt{\langle |x_{i+1} - x_i| \rangle^2 + \langle |y_{i+1} - y_i| \rangle^2}$ ($i = 1, \ldots, N-1$), and calculated then for each trajectory for all positions $i = 2, \ldots, N-2$ the largest diameter $S_d(t = i\Delta t)$ of the local convex hull of trajectory points $i-2, \ldots, i+2$. Representative time series $S_d(t)$ with their trajectories are shown in Fig. S6a.

Assuming stationarity and hence combining all values for $S_d$ of all trajectories from untreated cells into a single PDF revealed a non-Gaussian shape for $p(S_d)$ that suggests at least two states to be encoded in the trajectories (Fig. S6b). No significant difference was observed for trajectories from nocodazole-treated cells (see Fig. S6b).

In order to dissect the state with low mobility ('on') from states with a higher mobility ('off'), we employed the mean and standard deviation of $p(S_d)$, $\mu$ and $\sigma$, for defining a threshold $\theta$: For any excursion $S_d(t) \geq \theta$, the moving particle was rated to be in the high-mobility state (see Fig. S6a for examples). In the same analysis, also the periods in the low- and high-mobility states were quantified. Since the choice for $\theta$ is somewhat arbitrary, we tested values $\theta = \mu + k\sigma$ with $k = 1, 2, 3, 4$ (see also Fig. S6b). We observed, that the fraction of trajectories that did not show any switching grew considerably for $k = 3$ and $k = 4$ (cf. Fig. 3d in the main text). Therefore, we concentrated on thresholds $\theta = \mu + \sigma$ and $\theta = \mu + 2\sigma$.

Calculating the area under $p(S_d)$ in the range $0 \leq S_d \leq \mu + 2\sigma$ revealed, that about 82% of all $S_d$ values come from trajectory segments with a low mobility (low $S_d$ values). The remaining part of the PDF is due to at least one more state with a higher mobility that gives rise to larger $S_d$ values. For $\theta = \mu + \sigma$, the low-mobility area fraction is about 59%. Assuming only two states with a Markovian switching, as in the intermittent FBM model, the ratio of weights for the low- and high-mobility pools suggests a substantially longer mean residence time in the 'on'-state.

Evaluating the acquired residence times in terms of their PDFs revealed that both, $p(\tau_{\text{on}})$ and $p(\tau_{\text{off}})$, feature an exponential shape for $\theta = \mu + \sigma$ (Fig. 3c, main text) and $\theta = \mu + 2\sigma$ (Fig. S6c), irrespective of any treatment. Using different thresholds did not change the PDFs grossly (compare Fig. 3c to Fig. S6c). As anticipated, mean residence times in the 'on'-state were about threefold higher in both cases, allowing an estimate that particles spend on average about $\langle \tau_{\text{on}} \rangle / (\langle \tau_{\text{on}} \rangle + \langle \tau_{\text{off}} \rangle) \approx 75\%$ of their time in the slower 'on' state, in agreement with the above rationale.

It is worth noting at this point that the fairly short time series with only $N = 100$ positions certainly cannot accurately reveal the value of mean residence times if these are larger than $N\Delta t$. Yet, due to the Markovian nature of the switching process, one can obtain meaningful exponential PDFs of residence times that yield a significant estimate for the ratio $\langle \tau_{\text{on}} \rangle / \langle \tau_{\text{off}} \rangle$. In fact, applying the very same analysis to trajectories from simulations of the intermittent FBM model (see below for details) also revealed exponential PDFs for $p(\tau)$ with a ratio $\langle \tau_{\text{on}} \rangle / \langle \tau_{\text{off}} \rangle = 70 - 86\%$ when choosing thresholds in the range $\theta \in [\mu + \sigma, \mu + 2\sigma]$, in favorable agreement with the results obtained from our experimental data.

## G. Autocorrelation of squared increments

For an intermittent dichotomous process with rates $k_{\text{on}}$ and $k_{\text{off}}$, the ensemble-averaged autocorrelation function of fluctuations in the squared increments $\Delta r^2(t) = |\mathbf{r}(t + \Delta t) - \mathbf{r}(t)|^2$, i.e.

$$G(\tau) = \left\langle \frac{\langle \Delta r^2(t) \cdot \Delta r^2(t+\tau) \rangle_t - \langle \Delta r^2(t) \rangle_t^2}{\langle \Delta r^2(t) \rangle_t^2} \right\rangle_E , \tag{4}$$

should decay as $G(\tau) \sim \exp[-(k_{\text{on}} + k_{\text{off}})\tau]$ for sufficiently long trajectories [15]. Essentially, $G(\tau)$ describes how long a random walk is fueled by a homogenous PDF of steps with a given mean length before switching to a different mean step length. Consequently, pure and non-switching FBM trajectories yield $G(\tau) = 0$ for $\tau > \Delta t$ (Fig. S5b).

In line with the results obtained via the LCH analysis, we observed indeed a long-lasting decay of $G(\tau)$ for our experimental data (Fig. S5a). This result further substantiates the notion of a mobility change within individual trajectories. Moreover, our simulation data of an intermittent FBM random walk matched these experimental data very well, giving additional support to our reasoning. These simulations also confirmed that the seemingly unbounded decay of $G(\tau)$ is a consequence of the fairly slow switching that is not sampled well within short trajectories, leading to strongly fluctuating asymptotic zero lines in individual trajectories that are eventually ensemble-averaged. Simulating very long trajectories, the anticipated exponential form [15] was recovered.

### H. Simulations

To describe the experimental data, an intermittent FBM model was constructed. First, two-dimensional FBM trajectories with a fixed diffusion anomaly $\alpha_0$ were obtained via the Matlab routine *wfbm* with $i = 1, \ldots, N$ positions in each spatial dimension. From these trajectories, $N - 1$ successive step increments ($\Delta x$, $\Delta y$) were extracted and re-scaled to yield a TA-MSD with transport coefficient $K_\alpha = 0.004$ $\mu$m/s$^\alpha$, which is in the range of experimentally observed values. For compatibility with experiments, the time increment between successive positions was chosen to be $\Delta t = 100$ ms. To arrive at a heterogeneous, i.e. intermittent, FBM random walk in a second step, a stochastic switching between two modes of motion with rates $k_{\rm on}$ and $k_{\rm off}$ was implemented: While the previously obtained random walk steps were left unchanged in the 'on'-state, all steps in the 'off'-state were multiplied by a factor $s > 1$ to model an enhanced mobility. As a result, the transport coefficient of the FBM trajectory switched randomly from $K_\alpha$ to $sK_\alpha$ (or back) with rate $k_{\rm off}$ and $k_{\rm on}$, respectively. Due to this perturbation, the TA-MSD of the tracjectories showed a scaling with a slightly larger exponent $\langle\alpha\rangle$ than the value $\alpha_0$ imposed in the routine *wfbm*.

A very good matching to our experimental data with $N = 100$ positions (using an ensemble of $10^4$ trajectories) was observed for $s = 3.5$, $k_{\rm on} = 0.27$/s, and $k_{\rm off} = 0.0096$/s with $\alpha_0 = 0.5$ for untreated cells and $\alpha_0 = 0.3$ after depolymerizing microtubules. For $N = 500$, the rates $k_{\rm on}$ and $k_{\rm off}$ both needed to be chosen sixfold lower to match the experimental observations, indicating that trajectories with this length are a distinct subset of the entire data set.

### I. Discussion of alternative model descriptions

We have formulated a fairly simple two-state FBM process as a consistent and quantitative model description that captures the main features of the experimental data:

1. a subdiffusive scaling of individual TA-MSDs and of their ensemble averaged MSD
2. an ensemble- and time-averaged VACF with a significant anti-correlation that is very well described by the theoretical expression for subdiffusive FBM
3. a normalized step increment statistics that shows significant deviations from a simple Gaussian for short lag times but not for long lag times
4. a clear signature for at least two different modes of motion in the local-convex hull analysis of trajectories
5. a non-trivial decay of the autocorrelation of squared increments, indicating again a switching between at least two different modes of motion

Since more elaborate models might also be capable of capturing these experimental observations, we would like to briefly discuss here some of the most popular subdiffusion processes. Arguably these are continuous time random walks (CTRWs), obstructed diffusion (OD) in a fractal environment, scaled Brownian motion (SBM), and fractional Brownian motion (FBM).

CTRWs feature a weak ergodicity breaking, i.e. time- and ensemble-averaged MSDs have different scalings [16, 17]. Furthermore, CTRWs lack any appreciable anti-correlation in the normalized VACF in the unconfined case and also deviate significantly from the FBM prediction in the confined case [18]. Therefore, this class of processes is not consistent with observations 1 and 2, making it unlikely that they can properly capture the experimental findings. SBM can capture the anti-persistent characteristics in the VACF, but again shows a significant weak ergodicity breaking [19], rendering it inconsistent with observation 1. OD on the other hand is ergodic and also shows anti-correlated steps for a sufficiently high density of (almost) immobile obstacles [20]. In particular, obstacles need to occupy a volume fraction in the range $> 30\%$ (i.e. near to the percolation threshold), and have to adopt a fractal geometry. In addition, the arrangement of obstacles would have to result in a superb agreement of rescaled VACFs with the FBM prediction, which appears tricky in light of the previously reported distribution of turning angles [20]. While satisfying all points eventually might be possible with an OD model, a significant parameter fine-tuning will be needed, and it is questionable whether such a fine-tuned model can be compatible with the robust and dynamic state of living cells. Therefore, FBM-type random walks appear to be the most likely and straightforward models that satisfy observations 1 and 2.

In order to satisfy observations 3-5, some properties of the random walk need to undergo a change within individual trajectories. This could be, for example, a spatiotemporally varying transport coefficient (with the exception of arriving again at an SBM model). It is very likely that some or even all elaborate model variants of a diffusing diffusivity can, in combination with FBM-type random walks, lead to a consistent description of the experimental data. Using Occam's razor to arrive at the simplest but consistent model, we have implemented the mobility change by a basic

Markovian switching between just two states, which resulted already in a very good agreement with the experimental data. While the core features observed in experiments appear to be already included in our simple model, it may be illuminating to explore more refined and theoretically sophisticated models for describing the mobility changes. This, however, is beyond the scope of the current manuscript.

At this point we would like to emphasize that revealing the distinct features of different random-walk processes needs a combination of several measures rather than focussing on a single estimator. To this end, a broad palette of complementary analysis tools has been introduced and discussed in the literature (see e.g. [21–23]). For example, MSDs cannot tell whether the distribution of step sizes, $p(\chi)$, is Gaussian or not, whereas $p(\chi)$ holds no information about the temporal correlations of successive steps. The VACF probes such step correlations with explicit consideration of directional information (hence uncovering the memory kernel of the stochastic process), whereas the correlator of squared increments, $G(\tau)$, probes temporal changes of step lengths without directional information. These two correlators show significantly different shapes even for pure FBM processes, highlighting the fact that they probe complementary information. Understanding the diffusional motion in complex systems like living cells ulimately requires one to piece together the information gained from such different measures.

## II. SUPPLEMENTARY FIGURES

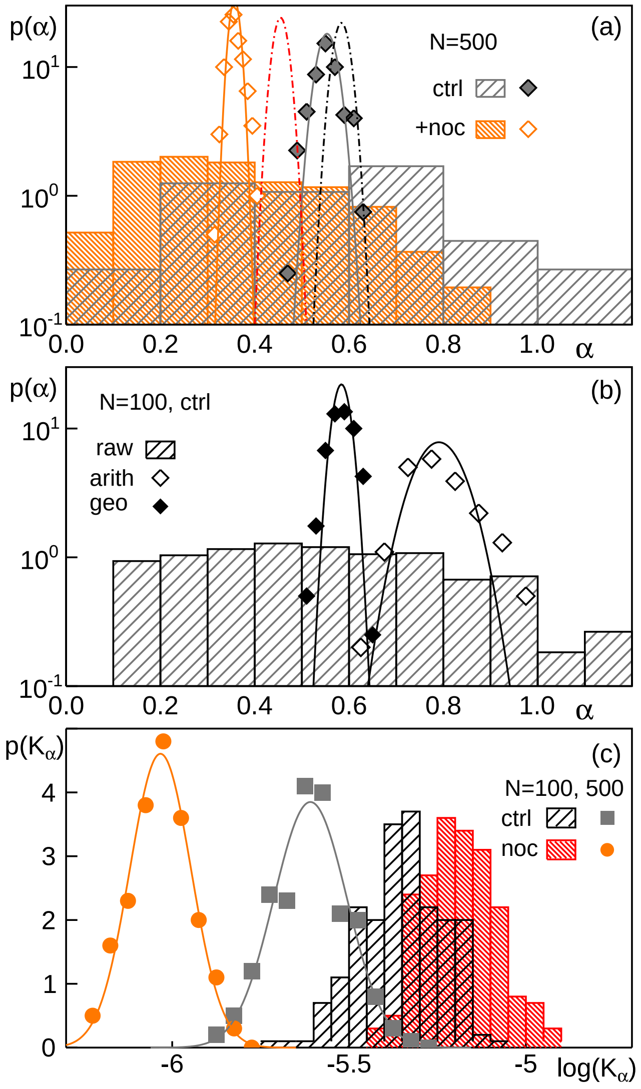


Figure S1: (a) In line with data shown in Fig. 1 in the main text, the PDF of anomaly exponents, $p(\alpha)$, as obtained from power-law fits on individual TA-MSDs of longer trajectories ($N = 500$) shows a fairly broad variation around a mean $\langle\alpha\rangle = 0.55$ in untreated cells (grey histogram). Nocodazole-treated cells have a similarly broad PDF (orange histogram) but feature a significantly lower mean (cf. Table I in the main text). Using the bootstrapping approach with geometric averaging (colored diamonds, full lines being best Gaussian fits) resulted in more narrow PDFs with the same mean anomaly. For better comparison with Fig. 1, Gaussian fits to the bootstrapping data for $N = 100$ in untreated and nocodazole-treated cells are reproduced as black and red dash-dotted lines, respectively. (b) For the representative case of short trajectories ($N = 100$) in untreated cells, PDFs $p(\alpha)$ obtained from raw TA-MSD fitting (hatched histogram) and bootstrapping with geometric or arithmetic averaging (filled and open diamonds, respectively) highlight a consistent over-estimation of the mean $\langle\alpha\rangle$ when using an arithmetic averaging (cf. also Table I in the main text). Full lines are best Gaussian fits to the bootstrapping data. (c) PDFs of the generalized transport coefficient $K_\alpha$, obtained by the bootstrapping method, roughly have a lognormal shape (full lines) in untreated and nocodazole-treated cells. Short trajectories ($N = 100$, histograms with color-coding as before) exhibit a small change upon disrupting microtubules whereas longer trajectories ($N = 500$) appear more sensitive to treatment with nocodazole (squares and circles). Supposedly, a low $K_\alpha$ facilitates the acquisition of longer trajectories, biasing the data for $N = 500$.

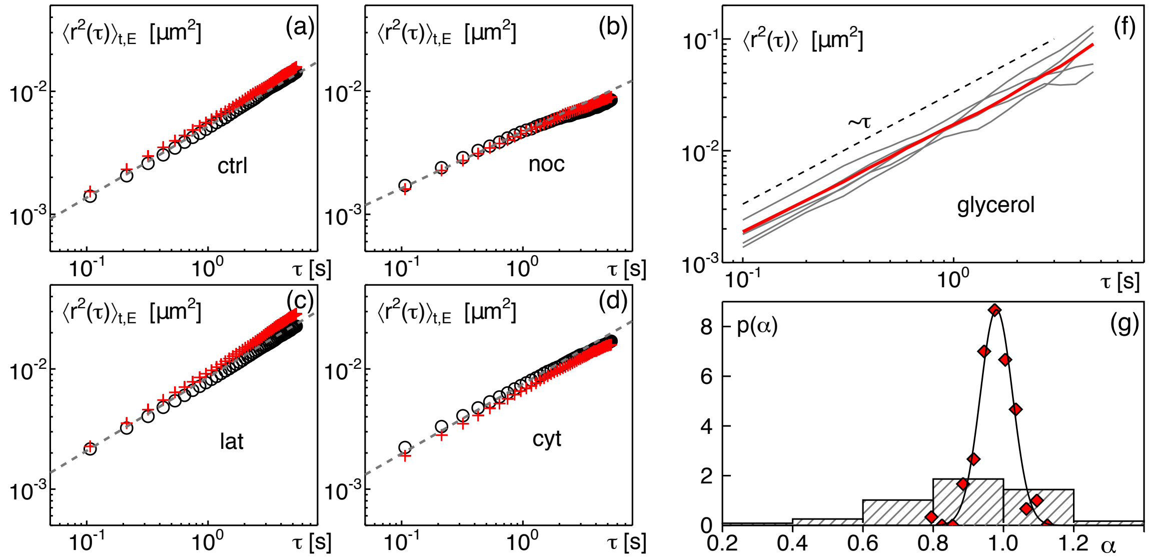


Figure S2: Representative geometrically averaged TA-MSDs (from trajectories with $N = 100$ positions) used for the bootstrapping approach (two examples, shown as black circles and red crosses) show no significant localization offsets at small lag times $\tau$ in (a) untreated, (b) nocodazole-, (c) latrunculin-, or (d) cytochalasin-treated cells. Grey dashed lines highlight the respective scaling given in Table I of the main text. This finding confirms and validates previously reported findings from comparable experiments [24] that had not been tested for perturbations by localization errors (see also Section E for a quantitative estimate of the small residual MSD offset). (f) SPT experiments on quantum dots in glycerol resulted in MSDs that were in favorable agreement with Brownian motion: Representative TA-MSDs (grey lines) and the ensemble mean $\langle r^2(\tau)\rangle_{t,E}$ (red line) follow the anticipated linear scaling (dashed scaling line). (g) The associated PDFs $p(\alpha)$, obtained from raw MSD fitting (grey hatched histogram) and via bootstrapping with geometric averaging (red symbols), feature a mean near to unity (highlighted by a Gaussian fit with mean $\langle\alpha\rangle = 0.98$ and standard deviation $\sigma = 0.05$, full line).

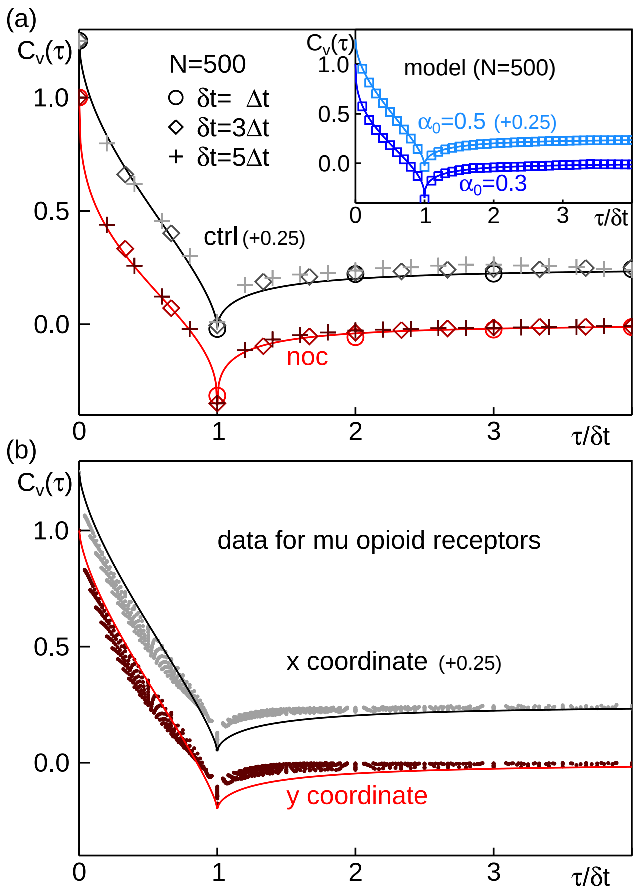


Figure S3: (a) The velocity autocorrelation function (VACF) for trajectories with $N = 500$ positions from untreated and nocodazole-treated cells agrees as well with the respective FBM prediction as the data for $N = 100$ (cf. Fig. 2 in the main text). Inset: The $N = 500$ trajectories for the intermittent FBM model also show a superb agreement with the prediction (full lines). (b) In contrast to quantum dots in the cytoplasm, the antipersistent motion of mu opioid receptors in the plasma membrane [25] show considerable deviations from the FBM prediction (full line).

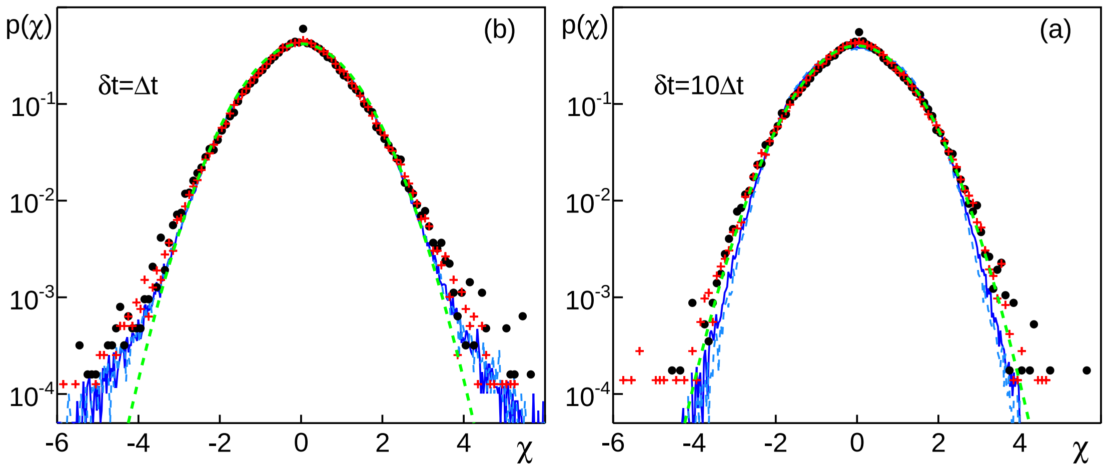


Figure S4: (a) The PDF of normalized increments $\chi$ from trajectories with $N = 100$ for a time lag $\delta t = \Delta t$ follows the anticipated Gaussian (green dashed line) for small $\chi$ but shows significant deviations at large $\chi$, suggesting a heterogeneous random walk process (black circles and red crosses: untreated and nocodazole-treated, respectively). The data are in good agreement with simulations of an intermittent FBM model ($\alpha_0 = 0.5$ and $\alpha_0 = 0.3$: coinciding light and dark blue lines). (b) For $\delta t = 10\Delta t$, experimental data and simulations follow a Gaussian for all $\chi$, i.e. deviations observed for $\delta t = \Delta t$ have subsided.

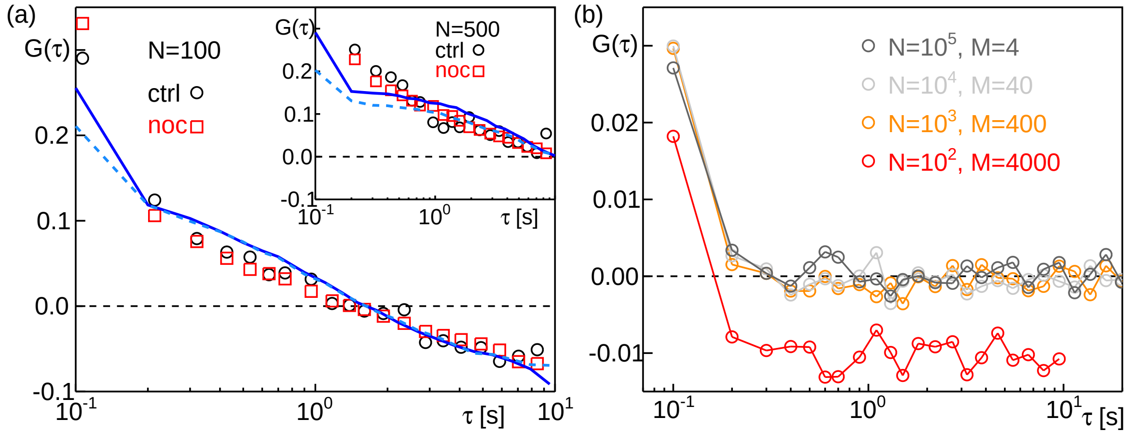


Figure S5: (a) The autocorrelation function of fluctuations in the squared increments, $G(\tau)$, of short trajectories ($N = 100$) shows a non-trivial decay for untreated and nocodazole-treated cells (black and red symbols, respectively), indicating a temporal change of transport parameters. These data are in very good agreement with simulation results of an intermittent FBM model (light and dark blue lines). Inset: Also for longer trajectories ($N = 500$), a non-trivial decay of $G(\tau)$ is observed that is well matched by simulation results of an intermittent FBM model. (b) For an ensemble of $M$ pure FBM trajectories with $\alpha = 0.7$ and $N$ positions the autocorrelation function of squared increments, $G(\tau)$ is basically zero beyond the basic time increment, $\tau = \Delta t$. For short trajectories ($N = 100$, red circles), a constant negative value is assumed due to statistical errors: Subtracting the baseline when calculuating $G(\tau)$ is only correct up to an uncertainty $\sim 1/\sqrt{N}$, yielding a constant $G(\tau \gg \Delta t) \sim -1/N$ that subsides for longer trajectories.

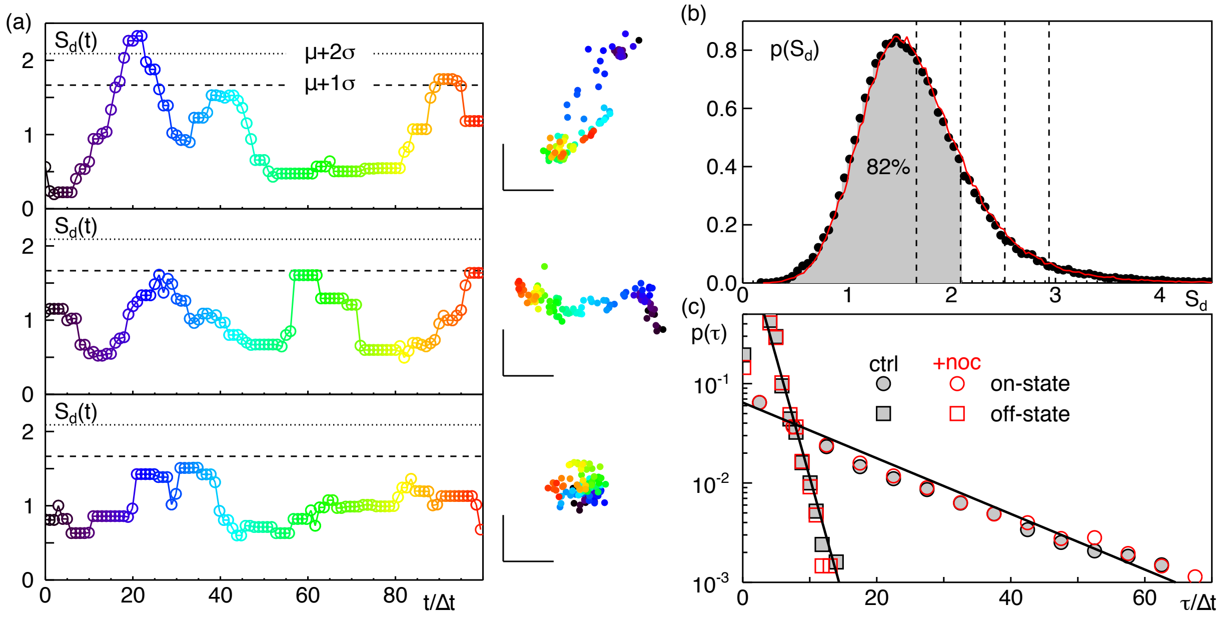


Figure S6: (a) Time series $S_d(t)$ of the diameter of the local convex hull (LCH) for three representative trajectories (progressing time being color-coded). Horizontal dashed and dotted lines mark thresholds $\mu + \sigma$ and $\mu + 2\sigma$ that were used for identifying the more mobile 'off' state (see Section F for details). Corresponding normalized trajectories (same temporal color-coding) are shown aside; horizontal and vertical scale bars have length 5. NB: The uppermost example is equivalent to Fig. 3b in the main text (apart from a global rotation). (b) The PDF $p(S_d)$ obtained from rescaled trajectories ($N = 100$) via the LCH analysis shows a non-symmetric shape around a marked peak. No significant difference is seen between untreated cells (black symbols) and nocodazole-treated cells (full red line). Vertical dashed lines indicate the threshold values $\theta = \mu + k\sigma$ ($k = 1, 2, 3, 4$) used for dissecting individual trajectories into 'on'- and 'off'-states (see Section F for details). Using $k = 2$, particles are seen to be in the low-mobility state for about 82% of all time points (grey area). (c) The PDF of residence times in the 'on'- and 'off'-states (representing a low and high mobility state, respectively), extracted from individual trajectories with a threshold $\theta = \mu + 2\sigma$ show an exponential decay (full lines), in agreement with results found for $\theta = \mu + \sigma$ (Fig. 3c, main text).

[1] L. Stadler and M. Weiss, New J. Phys. **19**, 113048 (2017).
[2] K. Speckner, L. Stadler, and M. Weiss, Phys. Rev. E **98**, 012406 (2018).
[3] L. Stadler, K. Speckner, and M. Weiss, Biophys. J. **115**, 1552 (2018).
[4] P. L. McNeil and E. Warder, J. Cell Sci. **88**, 669 (1987).
[5] M. A. Axelsson and G. Warren, Mol Biol Cell **15**, 1843 (2004).
[6] C. King, P. Sengupta, A. Seo, and J. Lippincott-Schwartz, bioRxiv (2019).
[7] G. Campagnola, K. Nepal, B. W. Schroder, O. B. Peersen, and D. Krapf, Sci. Rep. **5**, 17721 (2015).
[8] M. G. Gervasi, X. Xu, B. Carbajal-Gonzalez, M. G. Buffone, P. E. Visconti, and D. Krapf, J. Cell Sci. **131**, jcs215897 (2018).
[9] J.-Y. Tinevez, N. Perry, J. Schindelin, G. M. Hoopes, G. D. Reynolds, E. Laplantine, S. Y. Bednarek, S. L. Shorte, and K. W. Eliceiri, Methods **115**, 80 (2017).
[10] K. Jaqaman, D. Loerke, M. Mettlen, H. Kuwata, S. Grinstein, S. L. Schmid, and G. Danuser, Nat. Meth. **5**, 695 (2008).
[11] M. Weiss, Phys. Rev. E **100**, 042125 (2019).
[12] E. Kepten, I. Bronshtein, and Y. Garini, Phys. Rev. E **87**, 052713 (2013).
[13] Y. Lanoiselee and D. S. Grebenkov, Phys. Rev. E **96**, 022144 (2017).
[14] D. Arcizet, B. Meier, E. Sackmann, J. O. Rädler, and D. Heinrich, Phys. Rev. Lett. **101**, 248103 (2008).
[15] J. Cao, Phys. Rev. E **63**, 041101 (2001).
[16] Y. He, S. Burov, R. Metzler, and E. Barkai, Phys. Rev. Lett. **101**, 058101 (2008).
[17] A. Lubelski, I. Sokolov, and J. Klafter, Phys. Rev. Lett. **100**, 250602 (2008).
[18] S. Burov, J.-H. Jeon, R. Metzler, and E. Barkai, Phys. Chem. Chem. Phys. **13**, 1800 (2011).
[19] J.-H. Jeon, A. V. Chechkin, and R. Metzler, Phys. Chem. Chem. Phys. **16**, 15811 (2014).
[20] S. Sadegh, J. L. Higgins, P. C. Mannion, M. M. Tamkun, and D. Krapf, Phys. Rev. X **7**, 011031 (2017).
[21] F. Höfling and T. Franosch, Rep. Prog. Phys. **76**, 046602 (2013).
[22] R. Metzler, J.-H. Jeon, A. G. Cherstvy, and E. Barkai, Phys. Chem. Chem. Phys. **16**, 24128 (2014).
[23] K. Norregaard, R. Metzler, C. M. Ritter, K. Berg-Sørensen, and L. B. Oddershede, Chem. Rev. **117**, 4342 (2017).
[24] F. Etoc, E. Balloul, C. Vicario, D. Normanno, D. Lisse, A. Sittner, J. Piehler, M. Dahan, and M. Coppey, Nat. Mater. **17**, 740 (2018).
[25] M. J. Metz, R. L. Pennock, D. Krapf, and S. T. Hentges, Sci Rep **9**, 7297 (2019).
